# Supplementary material for: An Industry Evaluation of Embedding-based Entity Alignment
Source: arXiv:2010.11522 source file (2020-11-07)
Supplement: Supplementary file 1 [file 07-appendix.tex]

\begin{table}[ht]
    \centering
    \small
    
    \caption{Experimental results on D-W-15K-V2 dataset.}
    \begin{tabular}{l|l|l|p{0.8cm}<{\centering}p{0.8cm}<{\centering}p{0.8cm}<{\centering}|p{0.8cm}<{\centering}p{0.8cm}<{\centering}p{0.8cm}<{\centering}|p{0.8cm}<{\centering}p{0.8cm}<{\centering}p{0.8cm}<{\centering}}
        \Xhline{2\arrayrulewidth}
         \multicolumn{2}{c|}{} & \multirow{2}*{Models} & \multicolumn{3}{c|}{name stats (Hits@1)} & \multicolumn{3}{c|}{attr. stats (Hits@1)} & \multirow{2}*{Hits@1} & \multirow{2}*{Hits@5} & \multirow{2}*{MRR} \\
         \multicolumn{2}{c|}{} & & same & relev. & diff. & $<4$ & $4 - 10$ & $\geq10$ & & & \\
         \hline
         \parbox[t]{2mm}{\multirow{12}{*}{\rotatebox[origin=c]{90}{baseline}}} & \parbox[t]{2mm}{\multirow{4}{*}{\rotatebox[origin=c]{90}{tr-20\%}}} & BootEA & .868 & .902 & .753 & .721 & .822 & .912 & .818 & .922 & .864 \\
         & & MultiKE & .977 & .254 & .216 & .306 & .488 & .661 & .484 & .622 & .554 \\
         & & RDGCN & .942 & .934 & .305 & .330 & .734 & .827 & .629 & .756 & .687 \\
         & & RSN4EA & .718 & .718 & .579 & .536 & .663 & .753 & .650 & .797 & .717 \\
         \cline{2-12}
         & \parbox[t]{2mm}{\multirow{4}{*}{\rotatebox[origin=c]{90}{tr-4\%}}} & BootEA & .104 & .087 & .092 & .078 & .085 & .125 & .096 & .206 & .153 \\
         & & MultiKE & .975 & .217 & .088 & .159 & .440 & .647 & .413 & .513 & .467 \\
         & & RDGCN & .898 & .901 & .123 & .163 & .650 & .754 & .521 & .605 & .562 \\
         & & RSN4EA & .105 & .079 & .090 & .071 & .078 & .133 & .093 & .168 & .132 \\
         \cline{2-12}
         & \parbox[t]{2mm}{\multirow{4}{*}{\rotatebox[origin=c]{90}{tr-2\%}}} & BootEA & .024 & .022 & .030 & .028 & .025 & .026 & .026 & .073 & .051 \\
         & & MultiKE & .969 & .224 & .048 & .121 & .428 & .639 & .394 & .463 & .433 \\
         & & RDGCN & .900 & .895 & .107 & .147 & .636 & .761 & .513 & .582 & .547 \\
         & & RSN4EA & .026 & .015 & .031 & .025 & .021 & .034 & .027 & .056 & .044 \\
         \hline
         \parbox[t]{2mm}{\multirow{12}{*}{\rotatebox[origin=c]{90}{name-biased}}} & \parbox[t]{2mm}{\multirow{4}{*}{\rotatebox[origin=c]{90}{tr-20\%}}} & BootEA & .871 & .903 & .535 & .433 & .737 & .931 & .645 & .766 & .702 \\
         & & MultiKE & .978 & .285 & .080 & .085 & .230 & .318 & .185 & .335 & .261 \\
         & & RDGCN & .966 & .924 & .111 & .102 & .521 & .641 & .362 & .441 & .402 \\
         & & RSN4EA & .786 & .800 & .391 & .271 & .631 & .827 & .514 & .656 & .580 \\
         \cline{2-12}
         & \parbox[t]{2mm}{\multirow{4}{*}{\rotatebox[origin=c]{90}{tr-4\%}}} & BootEA & .733 & .817 & .358 & .260 & .633 & .802 & .554 & .642 & .596 \\
         & & MultiKE & .971 & .209 & .053 & .106 & .391 & .609 & .358 & .427 & .398 \\
         & & RDGCN & .956 & .905 & .076 & .128 & .616 & .766 & .491 & .544 & .518 \\
         & & RSN4EA & .198 & .185 & .087 & .051 & .147 & .228 & .138 & .228 & .182 \\
         \cline{2-12}
         & \parbox[t]{2mm}{\multirow{4}{*}{\rotatebox[origin=c]{90}{tr-2\%}}} & BootEA & .031 & .031 & .017 & .013 & .026 & .034 & .024 & .069 & .049 \\
         & & MultiKE & .968 & .195 & .027 & .093 & .389 & .617 & .360 & .404 & .388 \\
         & & RDGCN & .956 & .871 & .056 & .118 & .606 & .766 & .490 & .541 & .516 \\
         & & RSN4EA & .054 & .040 & .027 & .018 & .036 & .062 & .038 & .084 & .062 \\
         \hline
         \parbox[t]{2mm}{\multirow{12}{*}{\rotatebox[origin=c]{90}{attr-biased}}} & \parbox[t]{2mm}{\multirow{4}{*}{\rotatebox[origin=c]{90}{tr-20\%}}} & BootEA & .789 & .870 & .397 & .365 & .734 & .936 & .565 & .682 & .621 \\
         & & MultiKE & .975 & .358 & .078 & .145 & .488 & .767 & .334 & .459 & .398 \\
         & & RDGCN & .946 & .919 & .109 & .168 & .667 & .885 & .437 & .522 & .479 \\
         & & RSN4EA & .725 & .816 & .309 & .277 & .670 & .834 & .489 & .611 & .546 \\
         \cline{2-12}
         & \parbox[t]{2mm}{\multirow{4}{*}{\rotatebox[origin=c]{90}{tr-4\%}}} & BootEA & .704 & .819 & .337 & .245 & .622 & .800 & .538 & .611 & .574 \\
         & & MultiKE & .972 & .211 & .057 & .115 & .430 & .662 & .383 & .450 & .421 \\
         & & RDGCN & .922 & .908 & .091 & .133 & .630 & .798 & .501 & .557 & .529 \\
         & & RSN4EA & .192 & .213 & .083 & .056 & .156 & .228 & .141 & .232 & .185 \\
         \cline{2-12}
         & \parbox[t]{2mm}{\multirow{4}{*}{\rotatebox[origin=c]{90}{tr-2\%}}} & BootEA & .052 & .051 & .023 & .017 & .039 & .059 & .037 & .094 & .066 \\
         & & MultiKE & .968 & .229 & .041 & .104 & .426 & .651 & .384 & .449 & .421 \\
         & & RDGCN & .915 & .895 & .078 & .122 & .615 & .785 & .497 & .552 & .524 \\
         & & RSN4EA & .068 & .073 & .027 & .018 & .050 & .083 & .049 & .096 & .073 \\
        \Xhline{2\arrayrulewidth}
    \end{tabular}
    \label{tab:results}
\end{table}
